# Supplementary material for: Optical conductivity of multi-Weyl semimetals
Source: arXiv:1609.08566 source file (2017-04-27)
Supplement: Supplementary file 1 [file supplemental.pdf]

# Supplemental Material:
# Optical conductivity of multi-Weyl semimetals

Seongjin Ahn[1], E. J. Mele[2], and Hongki Min[1,2]
[1] Department of Physics and Astronomy, Seoul National University, Seoul 08826, Korea and
[2] Department of Physics and Astronomy, University of Pennsylvania, Philadelphia, PA 19104, USA

## I. CONTINUUM MODEL FOR EACH PHASE IN MULTI-WEYL SEMIMETALS

In this section, we discuss a continuum model for each phase in the phase diagram, including the transition point. For the calculation, we set $k_0 = 1/a$, $t_x = t_y = 4m_0$ and $t_z = 0.5m_0$ with $m_0 > 0$, and vary $-m_0 < m_z < m_0$ with other parameters fixed to induce various phases.

### A. WSM phase

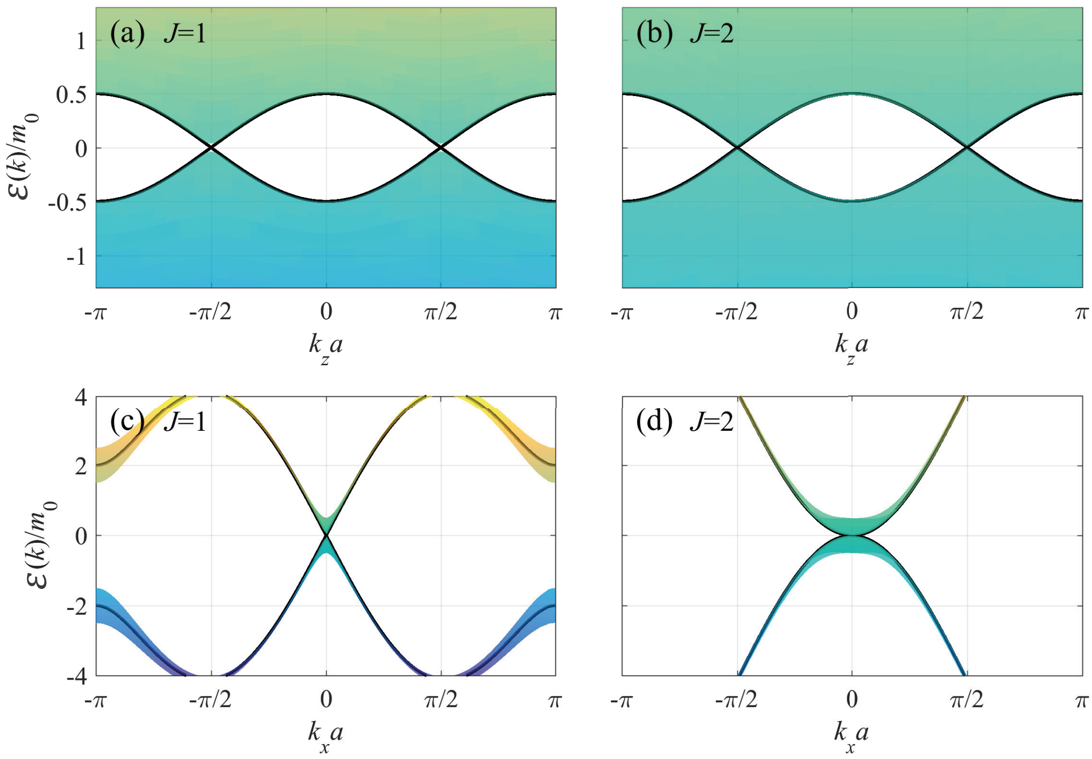


FIG. 1: Energy dispersions for the $J = 1$ and $J = 2$ lattice models in the WSM phase viewed from the $k_z$- and $k_x$-axes. Shaded regions represent the energy dispersions obtained by projecting them to (a), (b) the $k_z$-axis or to (c), (d) the $k_x$-axis at $k_y = 0$, in which each point of the dispersion is colored according to the energy scale, with yellow (blue) indicating higher (lower) values. The black solid lines are added to represent the energy dispersions across the Weyl node along (a), (b) the $k_z$-axis with $k_x = 0$ and (c), (d) the $k_x$-axis with $k_z = b$. Here, $m_z/m_0 = 0$ and $b = 0.5\pi/a$ are used for calculation.

First, consider a continuum model for the WSM phase. For $|m_z|/t_z < 1$ with $\cos(ba) \equiv m_z/t_z$, two Weyl points appear at $\boldsymbol{k} = \pm b\hat{\boldsymbol{z}}$, at which the conduction and valence bands touch at zero energy. Then, the Hamiltonian for $J = 1$ reduces to the form for Weyl semimetals:

$$H_1 \approx \hbar v_x k_x \sigma_x + \hbar v_y k_y \sigma_y \pm \hbar v_z q_z \sigma_z, \tag{1}$$

where $q_z = k_z \mp b$, $\frac{\hbar v_x}{a} = t_x$, $\frac{\hbar v_y}{a} = t_y$ and $\frac{\hbar v_z}{a} = t_z \sin(ba)$. Similarly, for $J = 2$, the Hamiltonian $H_2$ reduces to Eq. (1) of the main text with $J = 2$, where $\varepsilon_0 = \frac{1}{2} t_\parallel (k_0 a)^2$ with $t_x = t_y \equiv t_\parallel$ and $\frac{\hbar v_z}{a} = t_z \sin(ba)$. Note that the

two Weyl points located at $\boldsymbol{k} = \pm b\hat{\boldsymbol{z}}$ have opposite handedness $\chi = \pm 1$, representing the right-handed/left-handed chirality with Chern number $\chi J$.

Figure 1 shows the energy dispersion for the $J = 1$ and $J = 2$ lattice models in the WSM phase. As shown in Eq. (1) of the main text, the energy dispersion near the Weyl point along the $k_z$ direction with $k_x = k_y = 0$ is linear, while that along the $k_x$-$k_y$ directions with $k_z = 0$ is proportional to $k^J$. Note that there always appear multiple Weyl points in the Brillouin zone with the total chirality summing to zero, and in the lattice model we are considering, there are two Weyl nodes with opposite chiralities. Between the two Weyl points, the energy dispersion becomes flat along the $k_z$ direction at $k_x = k_y = 0$, showing a van Hove singularity, which gives rise to an interband transition peak in the optical conductivity, as shown in Fig. 2 in the main text.

## B. NI phase

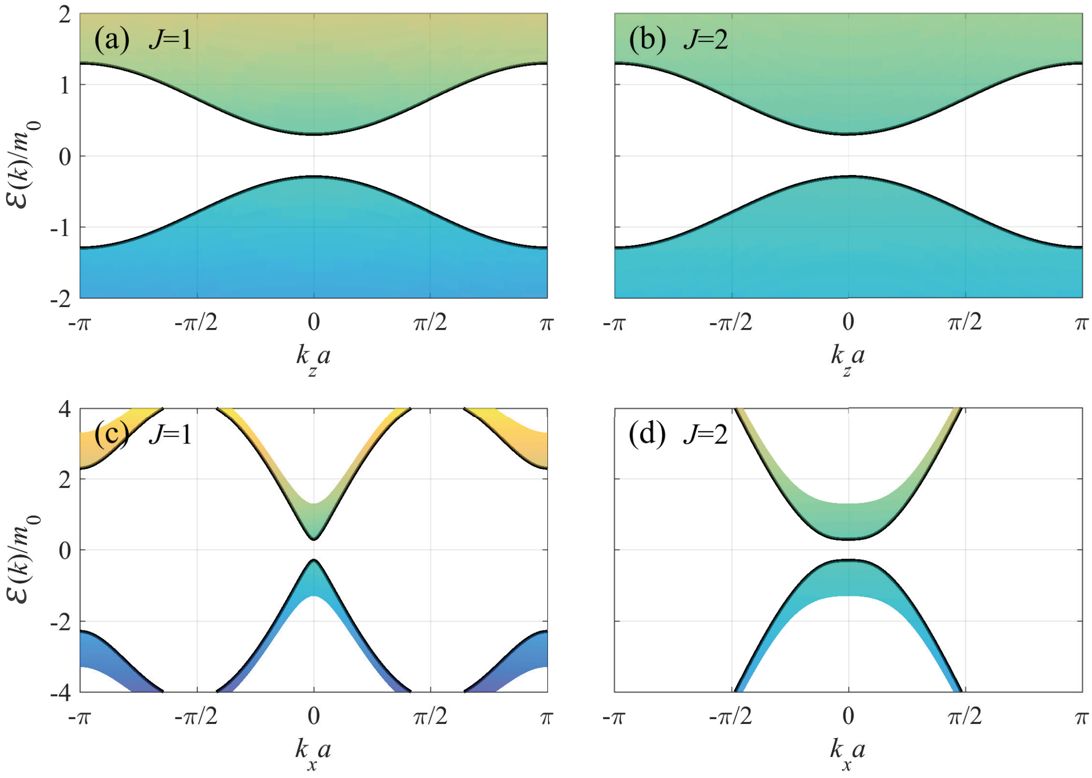


FIG. 2: Energy dispersions for the (a), (c) $J = 1$ and (b), (d) $J = 2$ lattice models in the NI phase viewed from the (a), (b) $k_z$- and (c), (d) $k_x$-axes with $k_y = 0$. Here, $m_z/m_0 = 0.8$ is used for the calculation.

For $m_z > t_z$, the mass term $M_z$ defined in Eq. (2) of the main text remains positive throughout the Brillouin zone, thus the system is in the trivial insulator phase. Near $\boldsymbol{k} = (0, 0, 0)$, $M_z$ can be approximated as

$$M_z \approx m_z - t_z + \frac{t_z a^2}{2} k_z^2 + \frac{m_0 a^2}{2} (k_x^2 + k_y^2). \tag{2}$$

Figure 2 shows the energy dispersions for the $J = 1$ and $J = 2$ lattice models with an energy gap of the size of $2\alpha$, where $\alpha = m_z - t_z$, which gives rise to a corresponding optical gap.

## C. 3D QAH phase

For $m_z < -t_z$, the mass term $M_z$ changes its sign in the Brillouin zone, generating a non-trivial insulating phase in contrast to the case of the NI phase. Near $\boldsymbol{k} = (0, 0, \pm\frac{\pi}{a})$, $M_z$ can be approximated as

$$M_z \approx m_z + t_z - \frac{t_z a^2}{2} q_z^2 + \frac{m_0 a^2}{2} (k_x^2 + k_y^2), \tag{3}$$

where $q_z = k_z \mp \frac{\pi}{a}$.

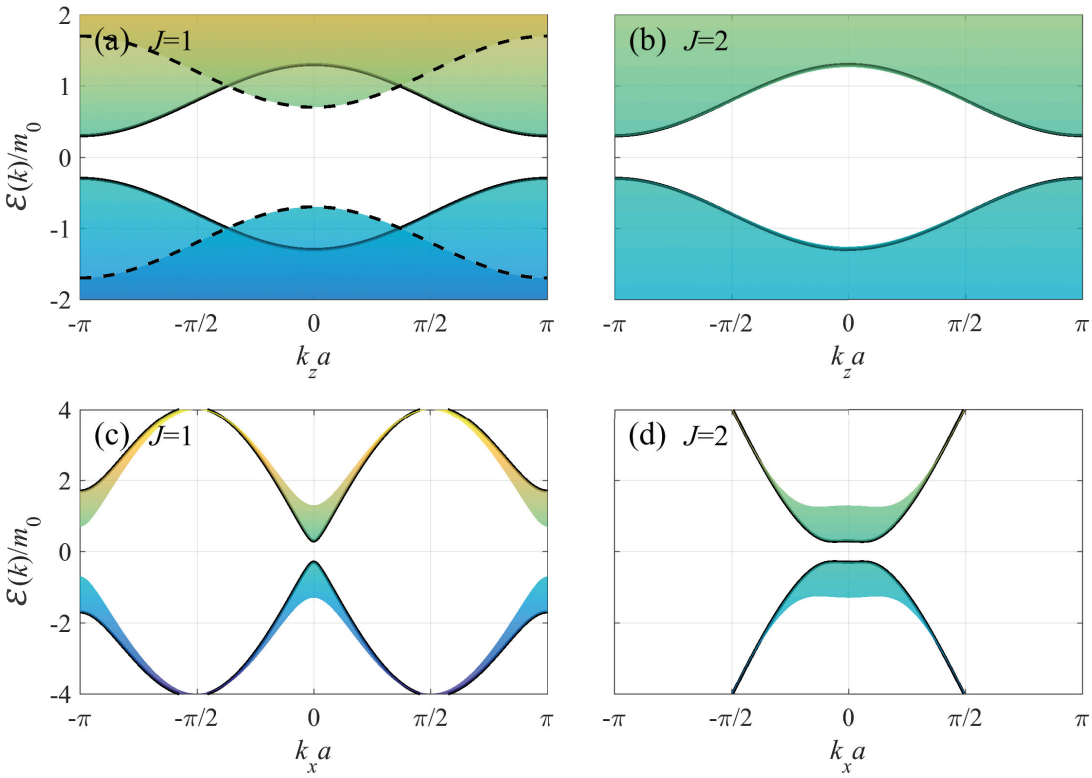


FIG. 3: Energy dispersions for the (a), (c) $J=1$ and (b), (d) $J=2$ lattice models in the 3D QAH phase viewed from the (a), (b) $k_z$- and (c), (d) $k_x$-axes with $k_y=0$. Here, $m_z/m_0=-0.8$ is used for the calculation. The dashed lines in (a) represent the energy dispersion along the $k_z$-axis with $k_x=\frac{\pi}{a}$ and $k_y=0$. Note that the interband transition between the dashed bands at $k_z=0$ corresponds to the second peak in $\sigma_{xx}(\omega)$, as shown in Fig. 3(a) in the main text.

Figure 3 shows the energy dispersion for the $J=1$ and $J=2$ lattice models in the 3D QAH phase. Because of the negative sign of the constant term $\alpha = m_z + t_z < 0$ in $M_z$, the 3D QAH phase has a different gap structure compared with the NI phase. Let $\gamma = \frac{m_0 a^2}{2} > 0$. It is easy to show that for $J=1$, if $\alpha \geq \alpha_{\mathrm{c}} = -\frac{\varepsilon_0^2}{2\gamma k_0^2}$, an energy gap of $2|\alpha|$ appears at $\boldsymbol{k} = (0,0,\pm\frac{\pi}{a})$, whereas if $\alpha < \alpha_{\mathrm{c}}$, a Mexican hat structure with the gap of $2\sqrt{2\alpha_{\mathrm{c}}\alpha - \alpha_{\mathrm{c}}^2}$ appears away from the $\boldsymbol{k}$ point. Note that in addition to $(k_x,k_y,k_z) = (0,0,\pm\frac{\pi}{a})$, there appear local minima at $(k_x,k_y,k_z) = (\pm\frac{\pi}{a},0,0)$ and $(0,\pm\frac{\pi}{a},0)$ in the $J=1$ 3D QAH phase, which result in an additional kink structure in the optical conductivity, as shown in Fig. 3(a) in the main text. For $J=2$, there is always a Mexican hat structure for $\alpha<0$ with a gap of $\frac{2|\alpha|}{\varepsilon_0(\varepsilon_0+\Gamma)}\sqrt{\varepsilon_0^2\Gamma^2 + (\varepsilon_0^2+\varepsilon_0\Gamma-\Gamma^2)^2}$, where $\Gamma = \gamma k_0^2$.

### D. Transition between the WSM and NI phases

At $m_z = t_z$, near $\boldsymbol{k} = (0,0,0)$, $M_z$ can be approximated as

$$M_z \approx \frac{t_z a^2}{2} k_z^2 + \frac{m_0 a^2}{2}(k_x^2 + k_y^2). \tag{4}$$

Figure 4 shows the energy dispersion for the $J=1$ and $J=2$ lattice models at the transition between the WSM and NI phases. Note that the low-energy dispersion along the $k_z$ direction with $k_x = k_y = 0$ is *quadratic*, while that along the $k_x$-$k_y$ directions with $k_z = 0$ is linear for $J=1$ and quadratic for $J>1$. As shown in the main text, the change in energy dispersion affects the optical conductivity, exhibiting a different characteristic frequency dependence compared with that in the WSM or NI phase.

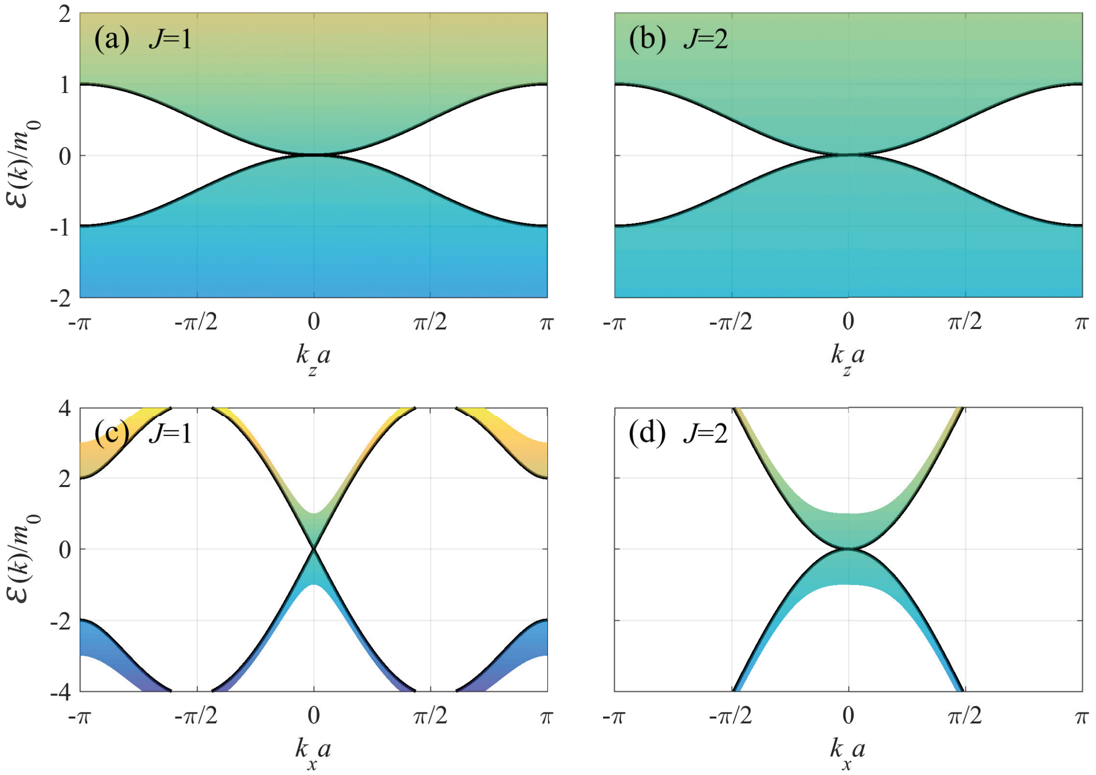


FIG. 4: Energy dispersions for the (a), (c) $J = 1$ and (b), (d) $J = 2$ lattice models at the transition between the WSM and NI phases viewed from the (a), (b) $k_z$- and (c), (d) $k_x$-axes with $k_y = 0$. Here, $m_z/m_0 = 0.5$ is used for the calculation.

### E. Transition between the WSM and 3D QAH phases

At $m_z = -t_z$, near $\boldsymbol{k} = (0, 0, \pm\frac{\pi}{a})$, $M_z$ can be approximated as

$$M_z \approx -\frac{t_z a^2}{2} q_z^2 + \frac{m_0 a^2}{2}(k_x^2 + k_y^2), \tag{5}$$

where $q_z = k_z \mp \frac{\pi}{a}$.

Figure 5 shows the energy dispersion for the $J = 1$ and $J = 2$ lattice models at the transition between the WSM and 3D QAH phases. Note that similar to the transition between the WSM and NI phases, the low-energy dispersion along the $k_z$ direction with $k_x = k_y = 0$ is *quadratic*, while that along the $k_x$-$k_y$ directions with $q_z = 0$ is linear for $J = 1$ and quadratic for $J > 1$. The change in energy dispersion affects the optical conductivity, exhibiting a different characteristic frequency dependence compared with that in the WSM or 3D QAH phase, as shown in Fig. 4 in the main text.

## II. ANALYTIC EXPRESSIONS OF OPTICAL CONDUCTIVITY FOR EACH PHASE

In this section, we present detailed derivations of the optical conductivities for multi-Weyl semimetals in various phases. We consider the following continuum Hamiltonian introduced in Eq. (5) of the main text that describes various phases such as normal insulators (NIs), Weyl semimetals (WSM) and 3D quantum anomalous Hall (QAH) states, along with the transition between them:

$$\begin{aligned} H &= \varepsilon_0 \left[ \left(\frac{k_-}{k_0}\right)^J \sigma_+ + \left(\frac{k_+}{k_0}\right)^J \sigma_- \right] + M_z \sigma_z, \\ M_z &= c_1 + c_2 \left(\frac{q_z}{k_0}\right)^n + c_3 \left[ \left(\frac{k_x}{k_0}\right)^2 + \left(\frac{k_y}{k_0}\right)^2 \right], \end{aligned} \tag{6}$$

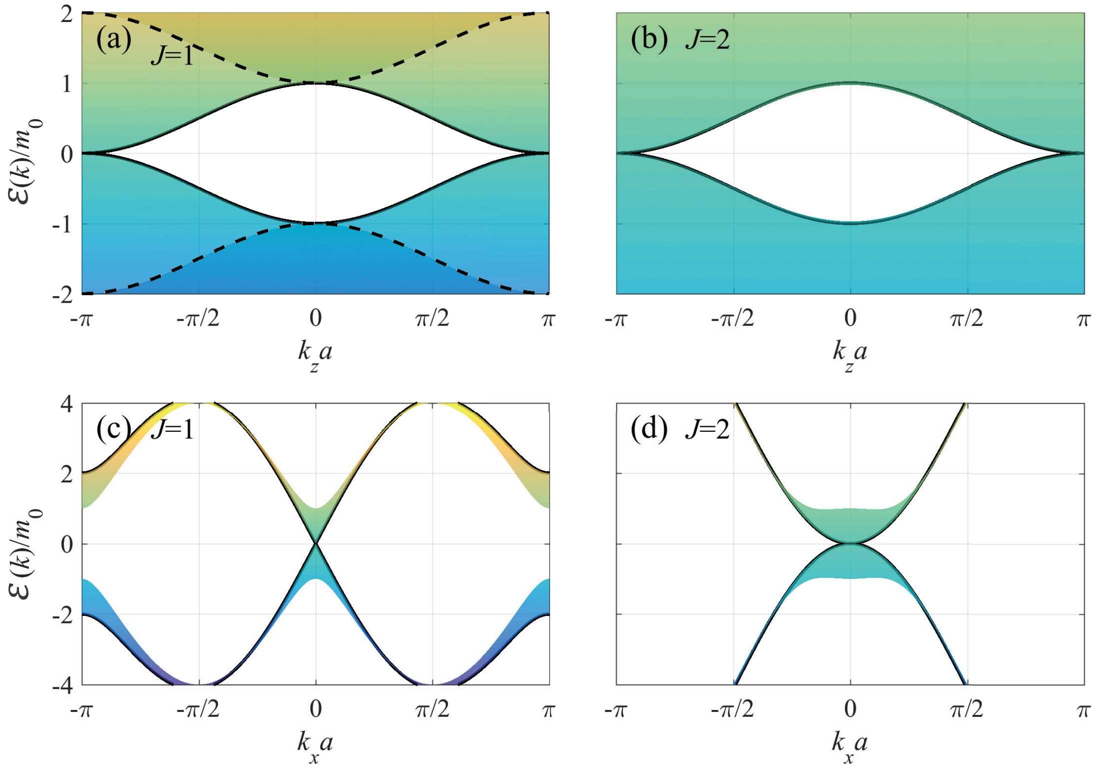


FIG. 5: Energy dispersions for the (a), (c) $J = 1$ and (b), (d) $J = 2$ lattice models at the transition between the WSM and 3D QAH phases viewed from the (a), (b) $k_z$- and (c), (d) $k_x$-axes with $k_y = 0$. Here, $m_z/m_0 = -0.5$ is used for the calculation.

where $\sigma_\pm = \frac{1}{2}(\sigma_x \pm i\sigma_y)$, $k_\pm = k_x \pm ik_y$, and $q_z$ is the effective wavevector along the $k_z$ direction defined in Eq. (6) of the main text. Note that for the WSM phase, $c_1 = 0$, $c_2 = \hbar v_z k_0$ and $c_3 = 0$ with $n = 1$, whereas for the insulator phases such as NI and 3D QAH, $c_1 = \alpha$, $c_2 = \beta k_0^2$ and $c_3 = \gamma k_0^2$ with $n = 2$. For the transition point, $c_1 = 0$, $c_2 = \beta k_0^2$ and $c_3 = \gamma k_0^2$ with $n = 2$.

### A. Longitudinal optical conductivity

Using Eq. (7) in the main text, we can obtain optical conductivities for multi-Weyl semimetals in the non-interacting limit. Note that for the longitudinal conductivity, $M_i^{ss'}(\boldsymbol{k})M_i^{s's}(\boldsymbol{k}) = |M_i^{ss'}(\boldsymbol{k})|^2$ $(i = x, y, z)$ is always real, thus the intraband and interband contributions of the real-part of the optical conductivity in the clean limit can be expressed as

$$\sigma_{ii}^{\text{intra}}(\omega) = -\frac{\pi e^2}{\hbar} \sum_{s=\pm} \int \frac{d^3k}{(2\pi)^3} \frac{\partial f_{s,\boldsymbol{k}}}{\partial \varepsilon_{s,\boldsymbol{k}}} |M_i^{ss}(\boldsymbol{k})|^2 \delta(\hbar\omega), \tag{7}$$

and

$$\sigma_{ii}^{\text{inter}}(\omega) = -\frac{\pi e^2}{\hbar} \int \frac{d^3k}{(2\pi)^3} \frac{f_{-,\boldsymbol{k}} - f_{+,\boldsymbol{k}}}{\varepsilon_{-,\boldsymbol{k}} - \varepsilon_{+,\boldsymbol{k}}} |M_i^{-+}(\boldsymbol{k})|^2 \delta(\hbar\omega + \varepsilon_{-,\boldsymbol{k}} - \varepsilon_{+,\boldsymbol{k}}), \tag{8}$$

at positive frequencies ($\omega > 0$).

Using this formula, it is straightforward to obtain the longitudinal optical conductivity for multi-Weyl semimetals. Because of the anisotropic energy dispersion, however, it is not trivial to obtain analytic expressions for the optical conductivity. In this section, we set $c_3 = 0$ (or $\gamma = 0$) for simplicity. This approximation works well for the Weyl phase because the linear term in $M_z$ corresponding to the linear dispersion along the $k_z$ direction is dominant over the quadratic mass term associated with $\gamma$ at low frequencies. In the insulating phases, however, the linear term is absent, and thus neglecting the quadratic $\gamma$ term is valid only when the effect of the band distortion associated with

nonzero $\gamma$ is small ($m_0 \ll t_x, t_y$). [See Sec. III(a) for the effect of $\gamma$ on the optical conductivity.] To avoid difficulties associated with anisotropic dispersions, we consider the following coordinate transformation

$$\begin{aligned} k_x &\to k_0 \left(\frac{\rho}{\varepsilon_0}\right)^{\frac{1}{J}} \cos\phi, \\ k_y &\to k_0 \left(\frac{\rho}{\varepsilon_0}\right)^{\frac{1}{J}} \sin\phi, \\ q_z &\to k_0 \left(\frac{z}{c_2}\right)^{\frac{1}{n}}, \end{aligned} \tag{9}$$

which transforms the Hamiltonian into the following linear form:

$$H = \rho(e^{-iJ\phi}\sigma_+ + e^{iJ\phi}\sigma_-) + (c_1 + z)\sigma_z. \tag{10}$$

Note that the transformed coordinates do not cover the lower hemisphere part (i.e., $q_z < 0$) when $n$ is an even number. We can avoid this problem by taking advantage of the inversion symmetry of the system $[H(q_z) = H(-q_z)$ for even $n]$, allowing us to get the right result by integrating over only the positive part of $q_z$. In the transformed coordinates, the energy dispersion is given by $E_\pm(\rho, z) = \pm E(\rho, z)$, where $E(\rho, z) = \sqrt{\rho^2 + (c_1 + z)^2}$. The corresponding eigenstate is given by

$$|+;\rho.\phi, z\rangle = \begin{pmatrix} \cos\frac{\theta}{2} \\ \sin\frac{\theta}{2} e^{iJ\phi} \end{pmatrix}, \tag{11a}$$

$$|-;\rho.\phi, z\rangle = \begin{pmatrix} -\sin\frac{\theta}{2} \\ \cos\frac{\theta}{2} e^{iJ\phi} \end{pmatrix}, \tag{11b}$$

where $\theta = \tan^{-1}\left(\frac{\rho}{c_1+z}\right)$. Note that $\cos\theta = \frac{c_1+z}{E(\rho,z)}$ and $\sin\theta = \frac{\rho}{E(\rho,z)}$.

The Jacobian $\mathcal{J}$ corresponding to this transformation is given by

$$\mathcal{J} = \begin{vmatrix} \frac{\partial k_x}{\partial \rho} & \frac{\partial k_x}{\partial \phi} & \frac{\partial k_x}{\partial z} \\ \frac{\partial k_y}{\partial \rho} & \frac{\partial k_y}{\partial \phi} & \frac{\partial k_y}{\partial z} \\ \frac{\partial q_z}{\partial \rho} & \frac{\partial q_z}{\partial \phi} & \frac{\partial q_z}{\partial z} \end{vmatrix} = \frac{k_0^3 \left(\frac{\rho}{\varepsilon_0}\right)^{\frac{2}{J}} \left(\frac{z}{c_2}\right)^{\frac{1}{n}}}{Jn\rho z} \equiv \mathcal{J}(\rho, z). \tag{12}$$

The velocity matrices $\hat{v}_i = \frac{1}{\hbar}\frac{\partial \hat{H}}{\partial k_i}$ can be expressed as

$$\hat{v}_x = \frac{J\varepsilon_0}{\hbar k_0}\left(\frac{\rho}{\varepsilon_0}\right)^{\frac{J-1}{J}} \begin{pmatrix} 0 & e^{-i(J-1)\phi} \\ e^{i(J-1)\phi} & 0 \end{pmatrix}, \tag{13a}$$

$$\hat{v}_y = \frac{J\varepsilon_0}{\hbar k_0}\left(\frac{\rho}{\varepsilon_0}\right)^{\frac{J-1}{J}} \begin{pmatrix} 0 & -ie^{-i(J-1)\phi} \\ ie^{i(J-1)\phi} & 0 \end{pmatrix}, \tag{13b}$$

$$\hat{v}_z = \frac{nc_2}{\hbar k_0}\left(\frac{z}{c_2}\right)^{\frac{n-1}{n}} \begin{pmatrix} 1 & 0 \\ 0 & -1 \end{pmatrix}. \tag{13c}$$

Then, the matrix elements of $M_i^{ss'}(\boldsymbol{k}) = \langle s, \boldsymbol{k}|\hbar\hat{v}_i|s', \boldsymbol{k}\rangle$ used in $\sigma_{xx}(\omega)$ and $\sigma_{zz}(\omega)$ are given by

$$M_x^{++}(\boldsymbol{k}) = \frac{J\varepsilon_0}{k_0}\left(\frac{\rho}{\varepsilon_0}\right)^{\frac{J-1}{J}} \frac{\rho\cos\phi}{E(\rho, z)}, \tag{14a}$$

$$M_x^{-+}(\boldsymbol{k}) = \frac{J\varepsilon_0}{k_0}\left(\frac{\rho}{\varepsilon_0}\right)^{\frac{J-1}{J}} \left[\frac{c_1 + z}{E(\rho, z)}\cos\phi - i\sin\phi\right], \tag{14b}$$

$$M_z^{++}(\boldsymbol{k}) = \frac{nc_2}{k_0}\left(\frac{z}{c_2}\right)^{\frac{n-1}{n}} \frac{c_1 + z}{E(\rho, z)}, \tag{14c}$$

$$M_z^{-+}(\boldsymbol{k}) = -\frac{nc_2}{k_0}\left(\frac{z}{c_2}\right)^{\frac{n-1}{n}} \frac{\rho}{E(\rho, z)}. \tag{14d}$$

After integrating over $\rho$ and $\phi$ in Eqs. (7) and (8), we can obtain the integral expressions with respect to $z$ for the longitudinal optical conductivity. The intraband part at zero temperature for the chemical potential $\mu \geq 0$ is then given by

$$\begin{aligned}
\sigma_{xx}^{\text{intra}}(\omega) &= \frac{\pi e^2}{\hbar}\int_{z_1}^{z_2} C_n dz \int_0^\infty d\rho \int_0^{2\pi} d\phi \frac{\mathcal{J}(\rho,z)}{(2\pi)^3}|M_x^{++}(\boldsymbol{k})|^2\delta(\hbar\omega)\delta\left(\mu - E(\rho,z)\right) \\
&= \frac{\pi e^2}{\hbar}\delta(\hbar\omega)\int_{z_1}^{z_2} C_n dz \int_0^\infty d\rho \frac{\mathcal{J}(\rho,z)}{(2\pi)^2}\left(\frac{J\varepsilon_0}{k_0}\right)^2\left(\frac{\rho}{\varepsilon_0}\right)^{\frac{2(J-1)}{J}}\frac{\rho^2}{2E^2(\rho,z)}\delta\left(\mu - E(\rho,z)\right) \\
&= \frac{e^2}{\hbar}\left(\frac{Jk_0\varepsilon_0^2}{8\pi n\mu}\right)\delta(\hbar\omega)\int_{z_1}^{z_2} C_n \frac{dz}{z}\left(\frac{z}{c_2}\right)^{\frac{1}{n}}\left(\frac{\rho_\mu(z)}{\varepsilon_0}\right)^2\Theta\left(\mu - |c_1+z|\right), \qquad (15a)\\
\sigma_{zz}^{\text{intra}}(\omega) &= \frac{\pi e^2}{\hbar}\int_{z_1}^{z_2} C_n dz \int_0^\infty d\rho \int_0^{2\pi} d\phi \frac{\mathcal{J}(\rho,z)}{(2\pi)^3}|M_z^{++}(\boldsymbol{k})|^2\delta(\hbar\omega)\delta\left(\mu - E(\rho,z)\right) \\
&= \frac{\pi e^2}{\hbar}\delta(\hbar\omega)\int_{z_1}^{z_2} C_n dz \int_0^\infty d\rho \frac{\mathcal{J}(\rho,z)}{(2\pi)^2}\left(\frac{nc_2}{k_0}\right)^2\left(\frac{z}{c_2}\right)^{\frac{2(n-1)}{n}}\frac{(c_1+z)^2}{E^2(\rho,z)}\delta\left(\mu - E(\rho,z)\right) \\
&= \frac{e^2}{\hbar}\left(\frac{nk_0c_2^2}{4\pi J\mu}\right)\delta(\hbar\omega)\int_{z_1}^{z_2} C_n \frac{dz}{z}\left(\frac{z}{c_2}\right)^{\frac{2n-1}{n}}\left(\frac{c_1+z}{\varepsilon_0}\right)^2\left(\frac{\rho_\mu(z)}{\varepsilon_0}\right)^{\frac{2(1-J)}{J}}\Theta\left(\mu - |c_1+z|\right), \qquad (15b)
\end{aligned}$$

where $\rho_\mu(z) = \sqrt{\mu^2 - (c_1+z)^2}$ and $\Theta(x)$ is the step function with $\Theta(x) = 1$ for $x > 0$ and 0 otherwise. The integration range is $(z_1, z_2)$=$(-\infty, \infty)$ for odd $n$, $(z_1, z_2)$=$(0, \infty)$ for even $n$ and $c_2 > 0$, and $(z_1, z_2)$=$(-\infty, 0)$ for even $n$ and $c_2 < 0$, and $C_n = 2$ for even $n$ and $C_n = 1$ for odd $n$. Here for the $\rho$ integration with a delta function, we use the relation $\delta(f(\rho)) = \frac{1}{|f'(\rho_0)|}\delta(\rho - \rho_0)$, where $f(\rho_0) = 0$.

For the interband part of optical conductivity, we set $\mu = 0$ for simplicity. Note that non-zero $\mu$ at zero temperature only gives rise to the Pauli blocking effect, thus the effect of non-zero $\mu$ can be taken into account by introducing the step function $\Theta(\hbar\omega - 2|\mu|)$ into the $\mu = 0$ result. [See Sec. III(c) for further discussion on the effect of finite $\mu$.] The interband part at zero temperature with $\mu = 0$ is given by

$$\begin{aligned}
\sigma_{xx}^{\text{inter}}(\omega) &= \frac{\pi e^2}{\hbar}\int_{z_1}^{z_2} C_n dz \int_0^\infty d\rho \int_0^{2\pi} d\phi \frac{\mathcal{J}(\rho,z)}{(2\pi)^3}\frac{|M_x^{-+}(\boldsymbol{k})|^2}{2E(\rho,z)}\delta\left(\hbar\omega - 2E(\rho,z)\right) \\
&= \frac{\pi e^2}{\hbar}\int_{z_1}^{z_2} C_n dz \int_0^\infty d\rho \frac{\mathcal{J}(\rho,z)}{(2\pi)^2}\frac{1}{2E(\rho,z)}\left(\frac{J\varepsilon_0}{k_0}\right)^2\left(\frac{\rho}{\varepsilon_0}\right)^{\frac{2(J-1)}{J}}\frac{1}{2}\left[\frac{(c_1+z)^2}{E^2(\rho,z)} + 1\right]\delta\left(\hbar\omega - 2E(\rho,z)\right) \\
&= \frac{e^2}{\hbar}\left(\frac{Jk_0}{32\pi n}\right)\int_{z_1}^{z_2} C_n \frac{dz}{z}\left(\frac{z}{c_2}\right)^{\frac{1}{n}}\left[\frac{(c_1+z)^2}{(\hbar\omega/2)^2} + 1\right]\Theta\left(\frac{\hbar\omega}{2} - |c_1+z|\right), \qquad (16a)\\
\sigma_{zz}^{\text{inter}}(\omega) &= \frac{\pi e^2}{\hbar}\int_{z_1}^{z_2} C_n dz \int_0^\infty d\rho \int_0^{2\pi} d\phi \frac{\mathcal{J}(\rho,z)}{(2\pi)^3}\frac{|M_z^{-+}(\boldsymbol{k})|^2}{2E(\rho,z)}\delta\left(\hbar\omega - 2E(\rho,z)\right) \\
&= \frac{\pi e^2}{\hbar}\int_{z_1}^{z_2} C_n dz \int_0^\infty d\rho \frac{\mathcal{J}(\rho,z)}{(2\pi)^2}\frac{1}{2E(\rho,z)}\left(\frac{nc_2}{k_0}\right)^2\left(\frac{z}{c_2}\right)^{\frac{2(n-1)}{n}}\frac{\rho^2}{E^2(\rho,z)}\delta\left(\hbar\omega - 2E(\rho,z)\right) \\
&= \frac{e^2}{\hbar}\left(\frac{nk_0}{4\pi J}\right)\left(\frac{c_2}{\hbar\omega}\right)^2\int_{z_1}^{z_2} C_n \frac{dz}{z}\left(\frac{z}{c_2}\right)^{\frac{2n-1}{n}}\left(\frac{\rho_\omega(z)}{\varepsilon_0}\right)^{\frac{2}{J}}\Theta\left(\frac{\hbar\omega}{2} - |c_1+z|\right), \qquad (16b)
\end{aligned}$$

where $\rho_\omega(z) = \sqrt{(\hbar\omega/2)^2 - (c_1+z)^2}$. In the subsequent sections, we present calculated optical conductivity for each phase.

### 1. *WSM phase*

For the WSM phase, $c_1 = 0$, $c_2 = \hbar v_z k_0$, $c_3 = 0$ and $n = 1$. From Eqs. (15) and (16), the longitudinal optical conductivity is given by

$$\sigma_{xx}(\omega) = \frac{g_{\rm N}}{24\pi}\frac{Je^2}{\hbar v_z}\left[\omega\Theta(\hbar\omega - 2|\mu|) + 4\omega_\mu^2\delta(\omega)\right], \tag{17a}$$

$$\sigma_{zz}(\omega) = \frac{g_{\rm N}}{24\pi}\frac{e^2 v_z}{\hbar v_\parallel^2}\left[A_{zz}^{\rm WSM}\left(\frac{\omega}{\omega_0}\right)^{\frac{2}{J}-1}\omega_0\Theta(\hbar\omega - 2|\mu|) + 4B_{zz}^{\rm WSM}\left(\frac{|\omega_\mu|}{\omega_0}\right)^{\frac{2}{J}}\omega_0^2\delta(\omega)\right], \tag{17b}$$

where $\varepsilon_0 = \hbar\omega_0 = \hbar v_\parallel k_0$, $\omega_\mu \equiv \mu/\hbar$, $A_{zz}^{\rm WSM} = \frac{3\sqrt{\pi}\Gamma(\frac{1}{J})}{2^{\frac{2}{J}}J^2\Gamma(\frac{1}{J}+\frac{3}{2})}$, and $B_{zz}^{\rm WSM} = \frac{3\sqrt{\pi}\Gamma(\frac{1}{J})}{4J\Gamma(\frac{1}{J}+\frac{3}{2})}$. Here, we introduced the number of nodes $g_{\rm N}$. In the derivation for $\sigma_{zz}$, we substitute $\frac{z}{\mu} = \sin\theta$ or $\frac{z}{\hbar\omega/2} = \sin\theta$, and use the relation $\int_0^{\pi/2} d\theta \cos^m\theta \sin^n\theta = \frac{1}{2}B(\frac{m+1}{2}, \frac{n+1}{2})$ where $B(m,n) = \frac{\Gamma(m)\Gamma(n)}{\Gamma(m+n)}$ is the beta function and $\Gamma(x) = \int_0^\infty dt\, t^{x-1}e^{-t}$ is the gamma function (See Ref. 18 in the main text.) Note that for $J = 1$, $A_{zz}^{\rm WSM}\big|_{J=1} = B_{zz}^{\rm WSM}\big|_{J=1} = 1$ and the result in Eq. (17) reduces to that of conventional Weyl semimetals.

The first term in Eq. (17) represents the interband transitions, which are forbidden at $\omega < 2|\omega_\mu|$ due to Pauli blocking, whereas the second term represents the intraband transition giving rise to the Drude peak at low frequencies. For the undoped case ($\mu = 0$), the result reduces to Eq. (8) in the main text.

### 2. *Insulator phase*

For both the NI and 3D QAH phases, $c_1 = \alpha$, $c_2 = \beta k_0^2$ and $n = 2$. As discussed, we set $c_3 = 0$ (or $\gamma = 0$) for simplicity. From now on, we consider only the undoped case, $\mu = 0$. The longitudinal optical conductivity is then obtained to be

$$\sigma_{xx}(\omega) = \frac{e^2}{\hbar}G_{xx}(\omega)\,(\hbar\omega - 2|\alpha|)^{\frac{1}{2}}\,\Theta(\hbar\omega - 2|\alpha|), \tag{18a}$$

$$\sigma_{zz}(\omega) = \frac{e^2}{\hbar}G_{zz}(\omega)\,(\hbar\omega - 2|\alpha|)^{\frac{1}{J}+\frac{3}{2}}\,\Theta(\hbar\omega - 2|\alpha|), \tag{18b}$$

where

$$G_{xx}(\omega) = \frac{J\left(16|\alpha|^2 + 4|\alpha|\hbar\omega + 9(\hbar\omega)^2\right)}{120\sqrt{2}\pi|\beta|^{\frac{1}{2}}(\hbar\omega)^2}, \tag{19a}$$

$$G_{zz}(\omega) = \frac{k_0\Gamma\left(\frac{1}{J}\right)}{2^{\frac{2}{J}+\frac{5}{2}}\sqrt{\pi}J^2\Gamma\left(\frac{1}{J}+\frac{5}{2}\right)}\frac{(|\beta|k_0^2)^{\frac{1}{2}}(\hbar\omega + 2|\alpha|)^{\frac{1}{J}}}{\varepsilon_0^{\frac{2}{J}}(\hbar\omega)^2}\,{}_2F_1\left(-\frac{1}{J}, \frac{3}{2}; \frac{1}{J}+\frac{5}{2}; \frac{2|\alpha| - \hbar\omega}{2|\alpha| + \hbar\omega}\right), \tag{19b}$$

and ${}_2F_1(a,b;c;z) = \frac{\Gamma(c)}{\Gamma(b)\Gamma(c-b)}\int_0^1 dt \frac{t^{b-1}(1-t)^{c-b-1}}{(1-tz)^a}$ is the hypergeometric function. Note that the analytic expressions for the longitudinal conductivities with $\gamma = 0$ have the same form for both NI and 3D QAH phases except for the sign of $\alpha$: $\alpha > 0$ for the NI phase and $\alpha < 0$ for the 3D QAH phase.

### 3. *Transition point*

For the transition point between the WSM and NI phases or between the WSM and 3D QAH phases, the analytical results can be obtained by taking the limit $\alpha \to 0$ in Eq. (18):

$$\sigma_{xx}(\omega) = \frac{e^2}{\hbar}A_{xx}\,(\hbar\omega)^{\frac{1}{2}}, \tag{20a}$$

$$\sigma_{zz}(\omega) = \frac{e^2}{\hbar}A_{zz}\,(\hbar\omega)^{\frac{2}{J}-\frac{1}{2}}, \tag{20b}$$

where

$$A_{xx} = \frac{3J}{40\sqrt{2}\pi|\beta|^{\frac{1}{2}}}, \tag{21a}$$

$$A_{zz} = \frac{k_0\Gamma\left(\frac{1}{J}\right)\left(|\beta|k_0^2\right)^{\frac{1}{2}}}{2^{\frac{2}{J}+2}J^2\Gamma\left(\frac{1}{4}\right)\Gamma\left(\frac{1}{J}+\frac{7}{4}\right)\varepsilon_0^{\frac{2}{J}}}. \tag{21b}$$

Here, we used ${}_2F_1(a,b;c;z) = {}_2F_1(b,a;c;z)$, ${}_2F_1(a,b;1+a-b;-1) = \frac{\Gamma(1+a-b)\Gamma\left(1+\frac{1}{2}a\right)}{\Gamma(1+a)\Gamma\left(1+\frac{1}{2}a-b\right)}$, and $\Gamma(x)\Gamma(1-x) = \frac{\pi}{\sin \pi x}$. (See Ref. 18 in the main text.)

### B. Transverse optical conductivity

From Eq. (7) in the main text, the Hall or transverse optical conductivity $\sigma_{xy}$ for $\mu = 0$ is given by

$$\sigma_{xy}(\omega) = -\frac{ie^2}{\hbar}\int \frac{d^3k}{(2\pi)^3}\frac{f_{+,\boldsymbol{k}} - f_{-,\boldsymbol{k}}}{\varepsilon_{+,\boldsymbol{k}} - \varepsilon_{-,\boldsymbol{k}}}\left[\frac{M_x^{+-}(\boldsymbol{k})M_y^{-+}(\boldsymbol{k})}{\hbar\omega + \varepsilon_{+,\boldsymbol{k}} - \varepsilon_{-,\boldsymbol{k}}} + \frac{M_x^{-+}(\boldsymbol{k})M_y^{+-}(\boldsymbol{k})}{\hbar\omega + \varepsilon_{-,\boldsymbol{k}} - \varepsilon_{+,\boldsymbol{k}}}\right]. \tag{22}$$

Here, in contrast to the longitudinal optical conductivity, we keep $c_3$ (or $\gamma$) for analytic expressions. Throughout this section, for brevity, the momentum and the energy are normalized by $k_0$ and $\varepsilon_0$, respectively, or equivalently we set $k_0 = \varepsilon_0 = 1$.

We consider the following coordinate transformation:

$$\begin{aligned} k_x &\to \rho^{\frac{1}{J}}\cos\phi, \\ k_y &\to \rho^{\frac{1}{J}}\sin\phi, \\ k_z &\to k_z, \end{aligned} \tag{23}$$

whose Jacobian is given by

$$\mathcal{J} = \frac{\rho^{\frac{2}{J}-1}}{J} \equiv \mathcal{J}(\rho). \tag{24}$$

In the transformed coordinate, the Hamiltonian becomes

$$H = \rho(e^{-iJ\phi}\sigma_+ + e^{iJ\phi}\sigma_-) + (c_1 + c_2 q_z^n + c_3\rho^{\frac{2}{J}})\sigma_z, \tag{25}$$

and the energy dispersion is given by $E_\pm(\rho, q_z) = \pm E(\rho, q_z)$, where

$$E(r, q_z) = \sqrt{\rho^2 + \left(c_1 + c_2 q_z^n + c_3\rho^{\frac{2}{J}}\right)^2}. \tag{26}$$

The corresponding eigenstate is given by

$$|+;\rho.\phi, q_z\rangle = \begin{pmatrix} \cos\frac{\theta}{2} \\ \sin\frac{\theta}{2}e^{iJ\phi} \end{pmatrix}, \tag{27a}$$

$$|-;\rho.\phi, q_z\rangle = \begin{pmatrix} -\sin\frac{\theta}{2} \\ \cos\frac{\theta}{2}e^{iJ\phi} \end{pmatrix}, \tag{27b}$$

where $\theta = \tan^{-1}\left(\frac{\rho}{m(\rho,q_z)}\right)$ and $m(\rho, q_z) = c_1 + c_2 q_z^n + c_3\rho^{\frac{2}{J}}$. Note that $\cos\theta = \frac{m(\rho,q_z)}{E(\rho,q_z)}$ and $\sin\theta = \frac{\rho}{E(\rho,q_z)}$.

The velocity matrices $\hat{v}_i = \frac{1}{\hbar}\frac{\partial \hat{H}}{\partial k_i}$ can be expressed as

$$\hat{v}_x = \frac{1}{\hbar}\begin{pmatrix} 2c_3\rho^{\frac{1}{J}}\cos\phi & J\rho^{\frac{J-1}{J}}e^{-i(J-1)\phi} \\ J\rho^{\frac{J-1}{J}}e^{i(J-1)\phi} & -2c_3\rho^{\frac{1}{J}}\cos\phi \end{pmatrix}, \tag{28a}$$

$$\hat{v}_y = \frac{1}{\hbar}\begin{pmatrix} 2c_3\rho^{\frac{1}{J}}\sin\phi & -iJ\rho^{\frac{J-1}{J}}e^{-i(J-1)\phi} \\ iJ\rho^{\frac{J-1}{J}}e^{i(J-1)\phi} & -2c_3\rho^{\frac{1}{J}}\sin\phi \end{pmatrix}. \tag{28b}$$

Then the matrix elements of $M_i^{ss'}(\boldsymbol{k}) = \langle s, \boldsymbol{k}|\hbar\hat{v}_i|s', \boldsymbol{k}\rangle$ used in $\sigma_{xy}(\omega)$ are given by

$$M_x^{+-}(\boldsymbol{k}) = J\left[\rho^{\frac{J-1}{J}}\left(\cos\theta\cos\phi + i\sin\phi\right)\right] - 2c_3\rho^{\frac{1}{J}}\sin\theta\cos\phi, \tag{29a}$$

$$M_y^{-+}(\boldsymbol{k}) = J\left[\rho^{\frac{J-1}{J}}\left(\cos\theta\sin\phi + i\cos\phi\right)\right] - 2c_3\rho^{\frac{1}{J}}\sin\theta\sin\phi. \tag{29b}$$

Note that

$$\int_0^{2\pi}\frac{d\phi}{2\pi}M_x^{+-}(\boldsymbol{k})M_y^{-+}(\boldsymbol{k}) = \int_0^{2\pi}\frac{d\phi}{2\pi}(M_x^{-+}(\boldsymbol{k})M_y^{+-}(\boldsymbol{k}))^* = iJ^2\rho^{\frac{2(J-1)}{J}}\left[\frac{J(c_1+c_2q_z^n)+(J-2)c_3\rho^{\frac{2}{J}}}{E(\rho,q_z)}\right]. \tag{30}$$

Then, from Eq. (22) the real part of the transverse optical conductivity is given by

$$\begin{aligned}\sigma_{xy}(\omega) &= -\frac{ie^2}{\hbar}\int_0^\infty d\rho\int_{-k_c}^{k_c}dk_z\int_0^{2\pi}d\phi\frac{\mathcal{J}(\rho)}{(2\pi)^3}\frac{1}{2E(\rho,q_z)}\left[\frac{M_x^{+-}(\boldsymbol{k})M_y^{-+}(\boldsymbol{k})}{\hbar\omega+2E(\rho,q_z)}+\frac{M_x^{-+}(\boldsymbol{k})M_y^{+-}(\boldsymbol{k})}{\hbar\omega-2E(\rho,q_z)}\right]\\ &= -\frac{e^2}{\hbar}\frac{1}{8\pi^2}\int_0^\infty\rho d\rho\int_{-k_c}^{k_c}dk_z\left[\frac{J(c_1+c_2q_z^n)+(J-2)c_3\rho^{\frac{2}{J}}}{E(\rho,q_z)}\right]\left[\frac{1}{E^2(\rho,q_z)-(\hbar\omega/2)^2}\right].\end{aligned} \tag{31}$$

Here, we introduce the momentum cutoff $k_c$ along the $k_z$ direction to prevent divergence of the integral. Using these results, we can obtain the real part of the transverse optical conductivity up to second order in $\omega$ as $\sigma_{xy}(\omega) \approx \sigma_{xy}^{(0)} + \sigma_{xy}^{(2)}(\omega)$, where

$$\begin{aligned}\sigma_{xy}^{(0)} &= -\frac{e^2}{\hbar}\frac{1}{8\pi^2}\int_{-k_c}^{k_c}dk_z\int_0^\infty\rho d\rho\frac{J(c_1+c_2q_z^n)+(J-2)c_3\rho^{\frac{2}{J}}}{E^3(\rho,q_z)}\\ &= \frac{e^2}{\hbar}\frac{1}{8\pi^2}\int_{-k_c}^{k_c}dk_z\left.\frac{J\left(c_1+c_2q_z^n+c_3\rho^{\frac{2}{J}}\right)}{E(\rho,q_z)}\right|_{\rho\to 0}^{\rho\to\infty},\end{aligned} \tag{32a}$$

$$\sigma_{xy}^{(2)}(\omega) = -\frac{e^2}{\hbar}\frac{(\hbar\omega)^2}{32\pi^2}\int_{-k_c}^{k_c}dk_z\int_0^\infty\rho d\rho\frac{J(c_1+c_2q_z^n)+(J-2)c_3\rho^{\frac{2}{J}}}{E^5(\rho,q_z)}. \tag{32b}$$

From now on, we recover $k_0$ and $\varepsilon_0$ for clarity.

### *1. WSM phase*

For the WSM phase, $c_1 = 0$, $c_2 = \hbar v_z k_0$, $c_3 = 0$ and $n = 1$. Then the Hall conductivity for a single Weyl node is given by

$$\sigma_{xy}^{(0)} = -\frac{e^2}{\hbar}\frac{J}{8\pi^2}\int_{-k_c}^{k_c}dk_z\mathrm{sgn}(v_zq_z). \tag{33}$$

Note that there always appear multiple Weyl points in the Brillouin zone with the total chirality summing to zero. Here, we consider the simplest case in which two Weyl nodes with opposite chirality are located at $\pm b\hat{\boldsymbol{z}}$, respectively. Assuming that the node with positive chirality is at $k_z = +b\hat{\boldsymbol{z}}$ and the negative one is at $k_z = -b\hat{\boldsymbol{z}}$ with $|b| < k_c$, we find

$$\sigma_{xy}^{(0)} = -\frac{e^2}{\hbar}\frac{J}{8\pi^2}\int_{-k_c}^{k_c}dk_z\left\{\mathrm{sgn}\left[v_z(k_z-b)\right]+\mathrm{sgn}\left[(-v_z)(k_z+b)\right]\right\} \tag{34}$$

$$= J\frac{e^2}{h}\frac{b}{\pi}. \tag{35}$$

Here, the first and second terms in the first line represent contributions from the positive and negative chirality nodes, respectively.

Similarly, we can obtain the dynamical part of the Hall conductivity. For a single Weyl node,

$$\begin{aligned}\sigma_{xy}^{(2)}(\omega) &= -\frac{e^2}{\hbar}\frac{J(\hbar\omega)^2}{32\pi^2}\int_{-k_c}^{k_c}dk_z\int_0^\infty\rho d\rho\frac{\hbar v_zq_z}{[\rho^2+(\hbar v_zq_z)^2]^{\frac{5}{2}}}\\ &= -\frac{e^2}{\hbar}\frac{J(\hbar\omega)^2}{96\pi^2}\int_{-k_c}^{k_c}dk_z\frac{\mathrm{sgn}\,(v_zq_z)}{(\hbar v_zq_z)^2}.\end{aligned} \tag{36}$$

Then, the total conductivity contributed from the two Weyl nodes is given by

$$\begin{aligned}\sigma_{xy}^{(2)}(\omega) &= -\frac{e^2}{\hbar}\frac{J\omega^2}{96\pi^2 v_z^2}\int_{-k_c}^{k_c} dk_z \left\{\frac{\text{sgn}\,[v_z(k_z-b)]}{(k_z-b)^2}+\frac{\text{sgn}\,[(-v_z)(k_z+b)]}{(k_z+b)^2}\right\} \\ &= \frac{e^2}{\hbar}\frac{J}{24\pi^2 v_z^2}\frac{b}{k_c^2-b^2}\omega^2. \end{aligned} \tag{37}$$

### *2. Insulator phase*

For both the NI and 3D QAH phases, $c_1=\alpha$, $c_2=\beta k_0^2$, $c_3=\gamma k_0^2$ and $n=2$. The static part of the Hall conductivity after the integration over $\rho$ is given by

$$\sigma_{xy}^{(0)} = \frac{e^2}{\hbar}\frac{1}{8\pi^2}\int_{-k_c}^{k_c} dk_z \begin{cases} 1-\text{sgn}[f(q_z)] & (J=1), \\ \frac{2\gamma k_0^2}{\sqrt{(\gamma k_0^2)^2+\varepsilon_0^2}} - 2\text{sgn}[f(q_z)] & (J=2), \end{cases} \tag{38}$$

where $f(q_z)=\alpha+\beta q_z^2$. Now, the integral is straightforward. In the NI phase ($\alpha>0$, $\beta>0$), $\text{sgn}[f(q_z)]=1$, thus

$$\sigma_{xy}^{(0)} = \frac{e^2}{\hbar}\begin{cases} 0 & (J=1), \\ \frac{k_c}{2\pi^2}\left(\frac{\gamma k_0^2}{\sqrt{(\gamma k_0^2)^2+\varepsilon_0^2}}-1\right) & (J=2), \end{cases} \tag{39}$$

whereas in the 3D QAH phase ($\alpha<0$, $\beta<0$), $\text{sgn}[f(q_z)]=-1$, and so

$$\sigma_{xy}^{(0)} = \frac{e^2}{\hbar}\begin{cases} \frac{k_c}{2\pi^2} & (J=1), \\ \frac{k_c}{2\pi^2}\left(\frac{\gamma k_0^2}{\sqrt{(\gamma k_0^2)^2+\varepsilon_0^2}}+1\right) & (J=2). \end{cases} \tag{40}$$

The results in Eq. (39) show that the static Hall conductivity $\sigma_{xy}^{(0)}$ in the NI phase is nonzero for $J=2$ in contrast to the corresponding lattice result, and that $\sigma_{xy}^{(0)}$ for the $J=2$ 3D QAH phase in Eq. (40) contains material dependent parameters such as $\gamma$ and $\varepsilon_0$. This is puzzling because the static Hall conductivity characterizing the topological state of the system should have a quantized value. The reason is that the static Hall conductivity for the continuum model is not properly regularized carrying an arbitrary residual value, thus it is not directly experimentally measurable but the difference in this quantity between different electronic states is. Since we know that the static part of the Hall conductivity in the NI phase is necessarily zero, we can directly obtain the residual conductivity to be $\sigma_{xy}^{(0)}$ in the NI phase. It is important to note that for the $J=2$ 3D QAH phase, after subtracting the residual conductivity, we obtain $\sigma_{xy}^{(0)}\big|_{\text{QAH}} \to \sigma_{xy}^{(0)}\big|_{\text{QAH}} - \sigma_{xy}^{(0)}\big|_{\text{NI}} = \frac{2e^2}{\hbar}\frac{k_c}{2\pi^2}$, as in Eq. (10) in the main text, which is quantized and consistent with the lattice result. (In general, the static Hall conductivity is proportional to the chirality so that $\sigma_{xy}^{(0)}\big|_{\text{QAH}} \to \frac{Je^2}{\hbar}\frac{k_c}{2\pi^2}$.) Note that the continuum model Hall conductivities presented in the figures throughout the paper (both numerical and analytic results) have this residual conductivity subtracted. In this sense, we choose the momentum cutoff along the $k_z$ direction as $k_c=\pi/a$ so that the properly subtracted static Hall conductivity in the 3D QAH phase has the same quantized value as in the lattice model.

Similarly, we can obtain the dynamical part of the Hall conductivity, whose leading order contribution is quadratic in frequency, i.e., $\sigma_{xy}^{(2)}=\frac{e^2}{\hbar}B_{xy}\omega^2$. In the NI phase,

$$B_{xy}^{\text{NI}} = k_0\left(\frac{\hbar}{\varepsilon_0}\right)^2 \begin{cases} -\frac{k_c\varepsilon_0^2}{96\pi^2\alpha k_0(\alpha+\beta k_c^2)} + \frac{8\alpha\gamma k_0^2-\varepsilon_0^2}{96\pi^2\sqrt{\alpha^3\beta}k_0}\tan^{-1}\left(\sqrt{\frac{\beta}{\alpha}}k_c\right) - \frac{\gamma k_0^2\tan^{-1}\left[2\sqrt{\frac{\beta k_c^2\gamma k_0^2}{4\alpha\gamma k_0^2+\varepsilon_0^2}}\right]}{6\pi^2\sqrt{\frac{\beta(4\alpha\gamma k_0^2+\varepsilon_0^2)}{\gamma}}} & (J=1), \\ \frac{\gamma k_0^2\varepsilon_0}{24\pi^2\alpha^2(\alpha+\beta k_c^2)}\sqrt{\frac{\alpha\left(\gamma^2k_0^4+\varepsilon_0^2\right)}{\beta k_0^2\varepsilon_0^2}}\left[\tan^{-1}\left(\sqrt{\frac{\beta}{\alpha}}k_c\right)(\alpha+\beta k_c^2)-k_c\sqrt{\alpha\beta}\right] & (J=2), \end{cases} \tag{41}$$

whereas in the 3D QAH phase,

$$B_{xy}^{\text{QAH}} = k_0\left(\frac{\hbar}{\varepsilon_0}\right)^2 \begin{cases} \frac{k_c\varepsilon_0^2}{96\pi^2 k_0\alpha(\alpha+\beta k_c^2)} - \frac{8\alpha\gamma k_0^2-\varepsilon_0^2}{96\pi^2\sqrt{\alpha^3\beta}k_0}\tan^{-1}\left(\sqrt{\frac{\beta}{\alpha}}k_c\right) & (J=1), \\ \frac{\gamma k_0^2\varepsilon_0}{24\pi^2\alpha^2(\alpha+\beta k_c^2)}\sqrt{\frac{\alpha\left(\gamma^2k_0^4+\varepsilon_0^2\right)}{\beta k_0^2\varepsilon_0^2}}\left[\tan^{-1}\left(\sqrt{\frac{\beta}{\alpha}}k_c\right)(\alpha+\beta k_c^2)-k_c\sqrt{\alpha\beta}\right] & (J=2). \end{cases} \tag{42}$$

Note that for $J = 2$, the dynamical part for the 3D QAH phase is given by the same form as that for the NI phase. In addition, $B_{xy}^{\mathrm{NI}}$ and $B_{xy}^{\mathrm{QAH}}$ are not zero, indicating that the system is a dynamical Hall insulator, even in the NI phase. Deep inside the NI (3D QAH) phase, however, $\lim_{\alpha\to\pm\infty} B_{xy} = 0$, thus the system becomes a trivial insulator (quantized Hall insulator) at finite frequencies.

#### 3. Transition point

For the transition point between the NI and WSM phases or between the 3D QAH and WSM phases, $c_1 = 0$, $c_2 = \beta k_0^2$, $c_3 = \gamma k_0^2$ and $n = 2$. Then, the transverse optical conductivity is given by the following form:

$$\sigma_{xy}^{\mathrm{NI|WSM}}(\omega) = \frac{e^2}{\hbar}\left[A_{xy}^{\mathrm{NI}} + C_{xy}^{\mathrm{NI|WSM}}\omega^{\nu}\right], \tag{43a}$$

$$\sigma_{xy}^{\mathrm{QAH|WSM}}(\omega) = \frac{e^2}{\hbar}\left[\frac{Jk_{\mathrm{c}}}{2\pi^2} + A_{xy}^{\mathrm{NI}} + C_{xy}^{\mathrm{QAH|WSM}}\omega^{\nu}\right], \tag{43b}$$

where $A_{xy}^{\mathrm{NI}}$ is a residual conductivity for the NI phase given by $A_{xy}^{\mathrm{NI}}\big|_{J=1} = 0$ for $J = 1$ and $A_{xy}^{\mathrm{NI}}\big|_{J=2} = \frac{k_{\mathrm{c}}}{2\pi^2}\left(\frac{\gamma k_0^2}{\sqrt{(\gamma k_0^2)^2+\varepsilon_0^2}} - 1\right)$ for $J = 2$, as shown in Eq. (39). As discussed in Sec. II B 2, the residual term $A_{xy}^{\mathrm{NI}}$ should be subtracted for the proper regularization, as shown in Eq. (11c) in the main text. Here, the exponent $\nu \approx 0.5$ is found numerically from Eq. (31) for $J = 1, 2$ with frequency independent coefficients $C_{xy}^{\mathrm{NI|WSM}}$ and $C_{xy}^{\mathrm{QAH|WSM}}$, respectively.

## III. EFFECTS OF THE $\gamma$ TERM, IMPURITIES, CHEMICAL POTENTIAL AND TILT ON THE OPTICAL CONDUCTIVITY

In this section, we discuss the effects of $\gamma$, impurities, chemical potential, and tilt on the optical conductivity, focusing on the validity of the characteristic frequency dependence described in this work. We show that the characteristic frequency dependence described in the main text is not altered below the frequency corresponding to the energy scale of the tilt or impurity potential. Here, we limit our discussion to the range of frequencies below the energy scale that the lattice effect becomes important and the Weyl Hamiltonian is no longer valid.

### A. $\gamma$ term

In the main text, we obtained the power-law in the longitudinal optical conductivities assuming $\gamma = 0$ in the insulating phases [Eq. (9) in the main text] and at the transition point [Eq. (11) in the main text]. Figure 6 shows the deviation of the power-law from that obtained within the $\gamma = 0$ approximation in the NI phase. For $J = 1$, the power-law is robust against the increase of $\gamma$ because the linear in-plane energy dispersion dominates over the quadratic term associated with $\gamma$. For $J = 2$, however, the deviation of the power-law is significant because the quadratic in-plane energy dispersion is comparable to the quadratic $\gamma$ term. At the transition point between the NI and WSM phases, the power-law is barely altered by $\gamma$ for both $J = 1$ and $J = 2$. The same conclusion holds for the QAH phase and the transition point between the QAH and WSM phases, because the gapped band structure is similar to that of the NI phase, unless a Mexican hat structure appears. Thus, we find that the deviation from the $\gamma = 0$ approximation is significant in the gapped phases for $J = 2$ but not in the gapless phases which extend to low frequency.

### B. Impurities

The effect of impurities or disorder can be taken into account in a simple form as a finite broadening term $\eta$ replacing the $0^+$ term in Eq. (6) in the main text for the Kubo formula. Figure 7 shows calculated optical conductivities for several values of $\eta$ which characterizes the strength of the impurity potential. Impurities affect the power-law in the optical conductivity below the frequency range set by the energy scale of the impurity potential. Above this energy scale, however, the characteristic power-law obtained in the clean limit remains valid. Note that simulating impurity effects with a broadening $\eta$ is approximate, and strong enough disorder can induce a phase transition, as shown in Ref. 12 in the main text, which is beyond the scope of this work.

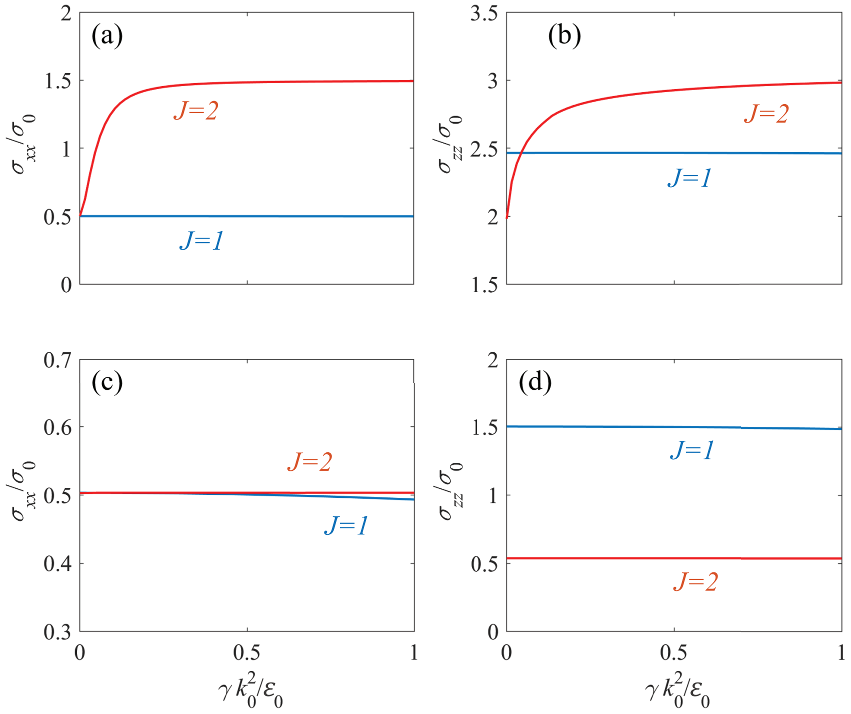


FIG. 6: Power-law exponent of $\sigma_{xx}$ and $\sigma_{zz}$ as a function of $\gamma k_0^2/\varepsilon_0$ (a), (b) in the NI phase and (c), (d) at the transition between the NI and WSM phases for $J = 1$ (blue) and $J = 2$ (red). For $J = 2$ in the NI phase, the deviation of the power-law from that obtained within the $\gamma = 0$ approximation is significant because the quadratic in-plane energy dispersion is comparable to the quadratic $\gamma$ term.

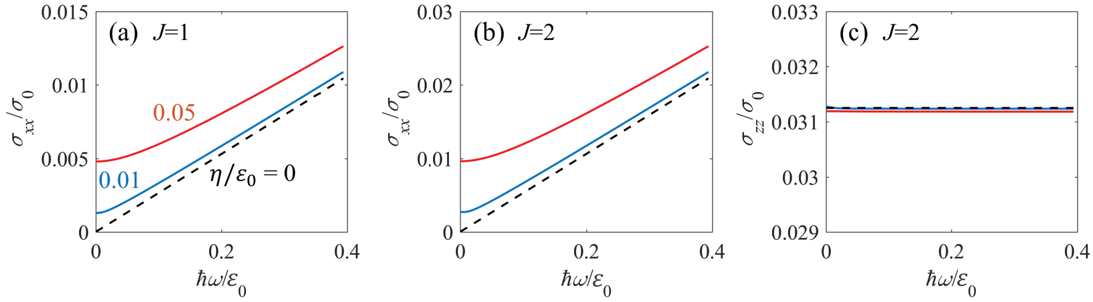


FIG. 7: Calculated longitudinal optical conductivities in the presence of disorder for (a) $J = 1$ and $J = 2$ in the (b) in-plane and (c) out-of-plane directions. Above the frequency scale set by the impurity potential, the characteristic frequency dependence presented in this work remains valid. Here, we set $\mu = 0$ and use several values of the broadening $\eta/\varepsilon_0 = 0, 0.01, 0.05$ for calculation.

### C. Chemical potential

Chemical potentials of m-WSMs do not need to stay at a Weyl node, and they vary depending on materials. Figure 8 shows calculated optical conductivities with zero and finite chemical potentials. As explained in the main text, a finite chemical potential $\mu$ away from a Weyl node produces a gap with a size of $2|\mu|$ due to Pauli blocking in interband transitions and a Drude peak near zero frequency from intraband transitions. Above the gap size, however, the optical conductivity follows the characteristic frequency dependence described in the main text.

### D. Tilt

In general, a Weyl node can be tilted breaking particle-hole symmetry. First, let us consider possible forms of a tilt Hamiltonian allowed for multi-Weyl nodes. As mentioned in the main text, multi-Weyl nodes are protected by

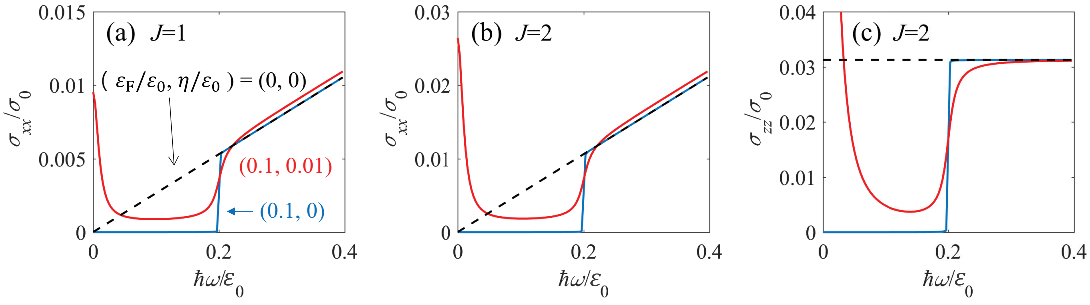


FIG. 8: Calculated longitudinal optical conductivities with chemical potentials $\mu = 0$ (dashed) and $\mu = 0.1\varepsilon_0$ (solid) for (a) $J = 1$ and $J = 2$ in the (b) in-plane and (c) out-of-plane directions. For finite $\mu$, in addition to results with $\eta = 0$ (blue), we present results with non-zero $\eta = 0.01\varepsilon_0$ (red) to induce a Drude peak with a finite width due to impurities. Above the frequency set by the gap with a size of $2|\mu|$, the optical conductivity follows the characteristic frequency dependence described in the main text.

point group symmetry. Assume that a multi-Weyl node is protected by an $n$-fold rotation along the $k_z$ axis, where $n = 2, 3, 4, 6$ is restricted by lattice. Then a tilt Hamiltonian near a node point $\boldsymbol{k} = 0$ is given by $H_\mathrm{t} = h(\boldsymbol{k})\sigma_0$. Following Fang *et al.* [1], we consider the functional form of $h(\boldsymbol{k})$ constrained by the $n$-fold rotational symmetry. Note that $H_\mathrm{t}$ is proportional to an identity matrix $\sigma_0$, thus $h(\boldsymbol{k})$ does not change its form by rotation, leading to the constraint $h(R_n\boldsymbol{k}) = h(\boldsymbol{k})$, where $R_n$ is the 3D rotation matrix for the $n$-fold rotation. Expressing $\boldsymbol{k}$ as $\boldsymbol{k} = (k_+, k_-, k_z)$ where $k_\pm = k_x \pm ik_y$, $R_n\boldsymbol{k}$ is given by

$$R_n\boldsymbol{k} = (k_+e^{i2\pi/n}, k_-e^{-i2\pi/n}, k_z). \tag{44}$$

Thus, from the constraint by the $n$-fold rotational symmetry, we have

$$h(k_+, k_-, k_z) = h(k_+e^{i2\pi/n}, k_-e^{-i2\pi/n}, k_z). \tag{45}$$

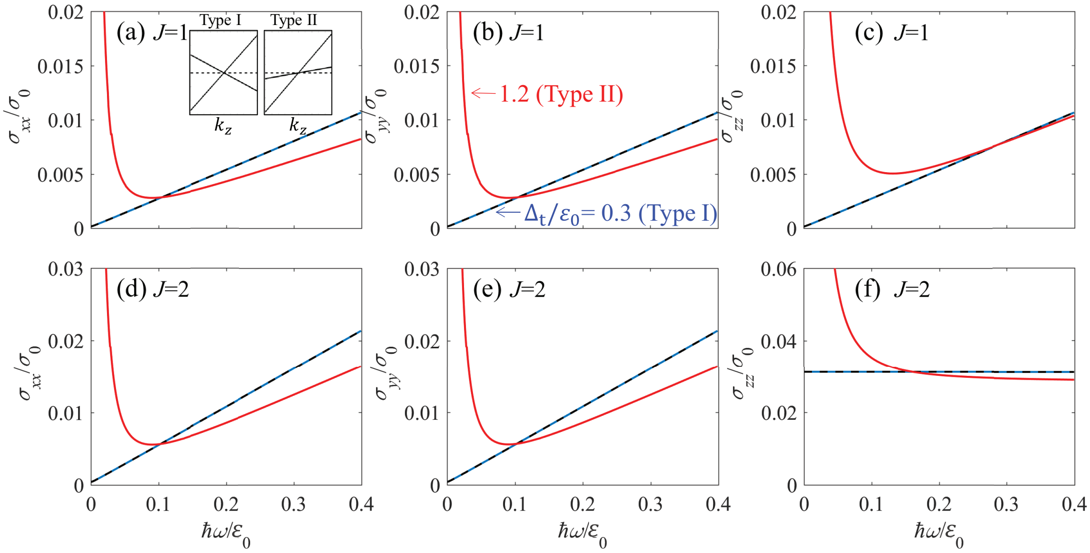


FIG. 9: Calculated longitudinal optical conductivities for (a)-(c) $J = 1$ and (d)-(f) $J = 2$ for several values of tilt $\Delta_\mathrm{t}/\varepsilon_0 = 0$ (black dashed), 0.3 (blue solid), 1.2 (red solid), where $\Delta_\mathrm{t} = \hbar v_\mathrm{t} k_0$. An inset to (a) shows the energy dispersion along the tilt direction. Here, $\eta = 0.001\varepsilon_0$ is used for the calculation.

To obtain an approximate effective Hamiltonian of the tilt term, assume an expansion of

$$h(k_+, k_-, k_z) = \sum_{n_1,n_2} C_{n_1n_2}k_+^{n_1}k_-^{n_2} + \hbar v_\mathrm{t}k_z, \tag{46}$$

where $C_{n_1n_2}$ is an expansion coefficient and $v_\mathrm{t}$ is the tilt velocity along the $k_z$ direction. Then from Eq. (45), we find $e^{i2\pi(n_1-n_2)/n} = 1$ or $n_1 - n_2 = 0$ (mod $n$) for non-vanishing $C_{n_1n_2}$. Thus the lowest order expansion of $k_+$ and $k_-$ is

given by $n_1 = n_2 = 1$ irrespective of $n$. Then the tilt Hamiltonian to the lowest order has a form of

$$h(\boldsymbol{k}) \approx C_{11}(k_x^2 + k_y^2) + \hbar v_{\rm t} k_z. \tag{47}$$

Here we used $k_+ k_- = k_x^2 + k_y^2$. This means that the in-plane tilt of multi-Weyl nodes cannot be linear, and the leading order tilt is a linear term along the direction of the rotational symmetry axis.

To understand the effect of tilt on the optical conductivity of m-WSMs, consider a tilt term given by $H_{\rm t} = \hbar v_{\rm t} k_z \sigma_0$. Figure 9 shows the optical conductivity of tilted multi-Weyl nodes. For both $J = 1$ and $J = 2$, tilt hardly affects the optical conductivity unless tilt is large enough that the system becomes type II [2] ($v_{\rm t} > v_{\parallel}$). When the system becomes type II Weyl semimetals, the Drude peak becomes significantly enhanced due to the formation of an electron-hole pocket whose size is comparable to the lattice scale ($\sim 1/a$). At sufficiently high frequencies, however, the optical conductivity recovers its original characteristic frequency behavior, as shown in Fig. 9.

[1] C. Fang, M. J. Gilbert, X. Dai, and B. A. Bernevig, Multi-Weyl Topological Semimetals Stabilized by Point Group Symmetry, Phys. Rev. Lett. **108**, 266802 (2012).
[2] A. A. Soluyanov, D. Gresch, Z. Wang, Q. S. Wu, M. Troyer, X. Dai, and B. A. Bernevig, Type II Weyl semimetals, Nature (London) **527**, 495 (2015).
